# Supplementary material for: Density dependence of the excitation gaps in an undoped Si/SiGe double-quantum-well heterostructure
Source: arXiv:2112.03138 ancillary file (2021-12-06)
Supplement: Supplementary file 1 [file Supplementary_Material.pdf]

# Supplementary Material for "Density dependence of the excitation gap in an undoped Si/SiGe double-quantum-well heterostructure"

D. Chen,[1] S. Cai,[1] N.-W. Hsu,[2] S.-H. Huang,[2] Y. Chuang,[2] E. Nielsen,[3] J.-Y. Li,[2,4] C. W. Liu,[2] T. M. Lu,[3] and D. Laroche[1,a]

[1] *Department of Physics, University of Florida, Gainesville, FL 32611, USA*

[2] *Department of Electrical Engineering and Graduate Institute of Electronic Engineering, National Taiwan University, Taipei 10617, Taiwan*

[3] *Sandia National Laboratories, Albuquerque, New Mexico 87185, USA*

[4] *Taiwan Semiconductor Research Institute, Hsinchu 30078, Taiwan*

(Dated: 25 October 2021)

[a] **Email of Author to whom correspondence should be addressed:** dlaroc10@ufl.edu

## CONTENTS

**I. Achieving Matched Density Between the Layers** 3

**II. Extraction of Excitation Gaps** 4

A. Arrhenius Plot Linear Fitting 5

**III. Schrödinger Poisson Simulations** 9

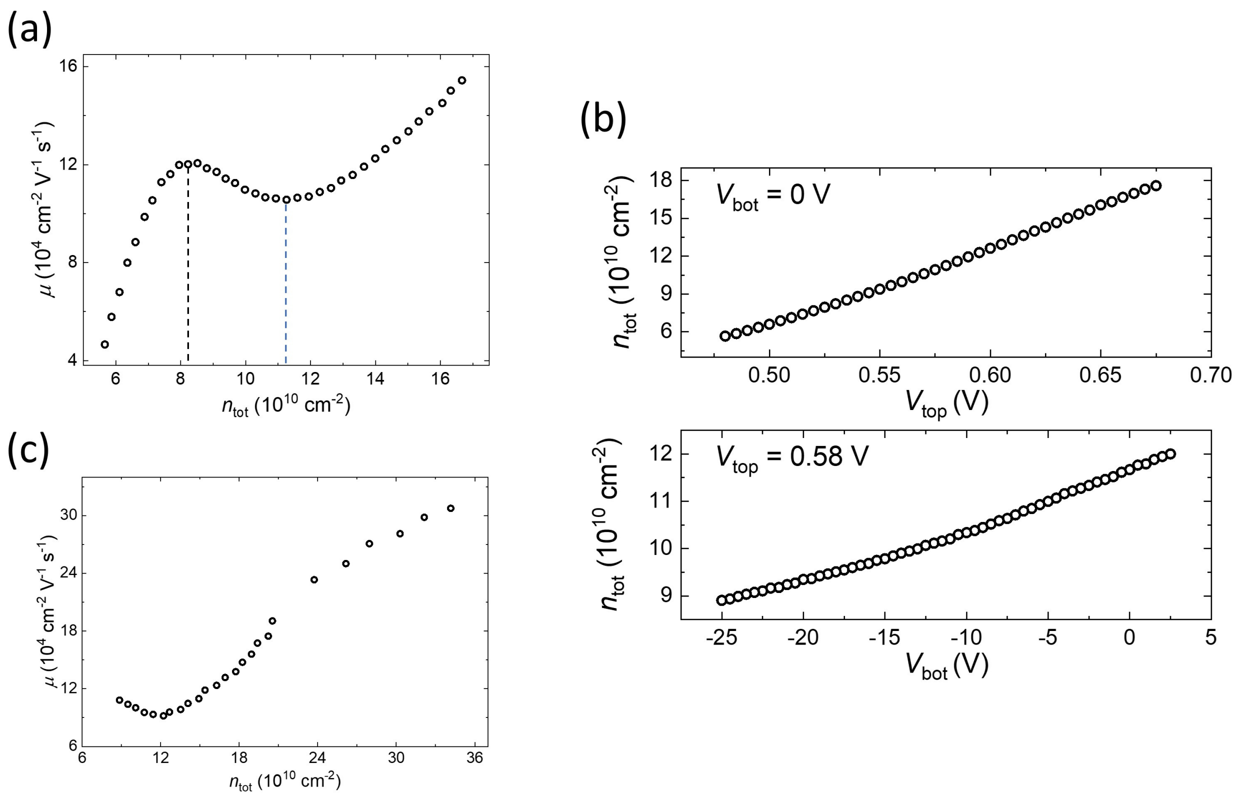


FIG. S1. (a) Total density vs mobility dependence. The dotted black line indicates $n_{\mathrm{crossover}}$. The dotted blue line indicates where $V_{\mathrm{top}} = 0.58$ V occurs. (b) Top Panel: Total density dependence vs top gate voltage with the bottom gate voltage set to 0. Bottom Panel: Total density dependence vs bottom gate voltage with a top gate voltage of 0.58 V. (c) Total density vs mobility dependence showcasing higher density values achieved at a different cooldown. The data was taken during a different cooldown than that of Fig. 2(c) of the main text, and that shown in panel (a).

## I. ACHIEVING MATCHED DENSITY BETWEEN THE LAYERS

The device's back gate was extensively used to tune the bilayer towards matched densities between the layers using the following procedure: First, the front gate voltage was increased, while keeping the back gate voltage at zero (Fig. S1(b)), in order to map out the mobility vs density curve shown in Fig. S1(a). The saturated bottom well density, corresponding to $n_{\mathrm{crossover}}$, is indicated by the black dotted line. Next, assuming that the bottom layer's density stays constant past the mobility peak, due to top layer screening, the bottom gate was modulated at constant front gate voltage as shown in Fig. S1(c). The initial top layer's density $n^0_{\mathrm{top}}$ is thus determined from $n^0_{\mathrm{top}} = n_{\mathrm{tot}} - n_{\mathrm{crossover}}$. Subsequent changes in the bottom gate will not modify $n^0_{\mathrm{top}}$ due to

bottom layer screening. Thus, the new bottom layer density is determined by $n_{\text{bot}} = n_{\text{tot}} - n^0_{\text{top}}$. Collating the behavior of the top (bottom) gates with respect to the bottom (top) wells' densities, matched density between the layers can be reasonably achieved, $n_{\text{tot}} = 2n_{\text{top}} = 2n_{\text{bot}}$, within 6%. It is important to note that each gate predominantly affects the nearest well but also slightly affects the farther well, modifying the density by less than 4% over the simulated range. Since the density of the bottom layer is initially much larger than that of the top layer, the back gate voltages are generally negative in order to reduce the bottom layer's density to reach the matched density regime. The densities of each layer in the matched density case are given in the following table. The starred voltages represent the values used when extracting $\Delta_1$.

TABLE S.I. Matched Density Case

| $V_{\text{top}}$ (V) | $V_{\text{bot}}$ (V) | $n_{\text{tot}}$ ($10^{10}$ cm$^{-2}$) | $n_{\text{top}}$ ($10^{10}$ cm$^{-2}$) | $n_{\text{bot}}$ ($10^{10}$ cm$^{-2}$) | % Difference |
|---|---|---|---|---|---|
| 0.62 | -26.525 | 11.24 | 5.77 | 5.47 | 5.47 |
| 0.63 | -18.976 | 12.79 | 6.43 | 6.36 | 1.22 |
| 0.64 | -12.368 | 14.14 | 7.11 | 7.03 | 1.18 |
| 0.65 | -6.375 | 15.37 | 7.84 | 7.53 | 4.04 |
| 0.66 | -1.375 | 16.66 | 8.44 | 8.22 | 2.74 |
| 0.67 | 3.457 | 17.7 | 9.09 | 8.61 | 5.5 |
| 0.62* | -26.525* | 11.57 | 5.77 | 5.8 | 0.53 |
| 0.625* | -22.613* | 12.24 | 6.08 | 6.16 | 1.33 |
| 0.63* | -18.976* | 13.05 | 6.43 | 6.62 | 2.76 |
| 0.64* | -12.368* | 14.45 | 7.11 | 7.34 | 3.16 |

## II. EXTRACTION OF EXCITATION GAPS

The quantum Hall excitation gaps, shown in Fig. 3 of the letter, are extracted from the temperature dependence of the $\rho_{xx}$ minima. The temperatures probed, [100 mK - 1.1 K], were adjusted and maintained using PID controllers and sufficient time was given for the device to reach thermal equilibrium, as indicated by $\rho_{xx}$ plateauing at each value. (Fig. S2)

After averaging the values of $\rho_{xx}$ and $T$ at the end of each plateau, an Arrhenius plot was constructed. At low temperatures, non-linear behavior is shown due to interstitial hopping. The

linear part of the plot was systematically determined and fitted to an activation model using the following general procedure.

## A. Arrhenius Plot Linear Fitting

The algorithm was coded to determine the interval in the Arrhenius plot that is the most linear while assuming interstitial hopping occurs at low temperatures. With this in mind, the data sets were split based on whether we were considering $\nu_{\text{tot}} = 1$ or $\nu_{\text{tot}} = 2$ as well as whether we were in the variable imbalanced or matched density regimes, giving us four data sets. For each set, the maximum slope change as well as the starting temperature interval were defined to be the same. The starting temperature interval was determined after visual inspection of each data set. It is important to note that data points higher than .9 K were disregarded as the quantum Hall minima becomes too weak to identify at higher temperatures.

The activation gap was determined from the following iterative procedure. First, the slope of the defined starting temperature interval is calculated and is called the original slope. Subsequently, 2 new slopes are calculated by adding one data point to the left or to the right of the fitting interval. If the percent change between the new slopes and the original slope is less than the pre-determined

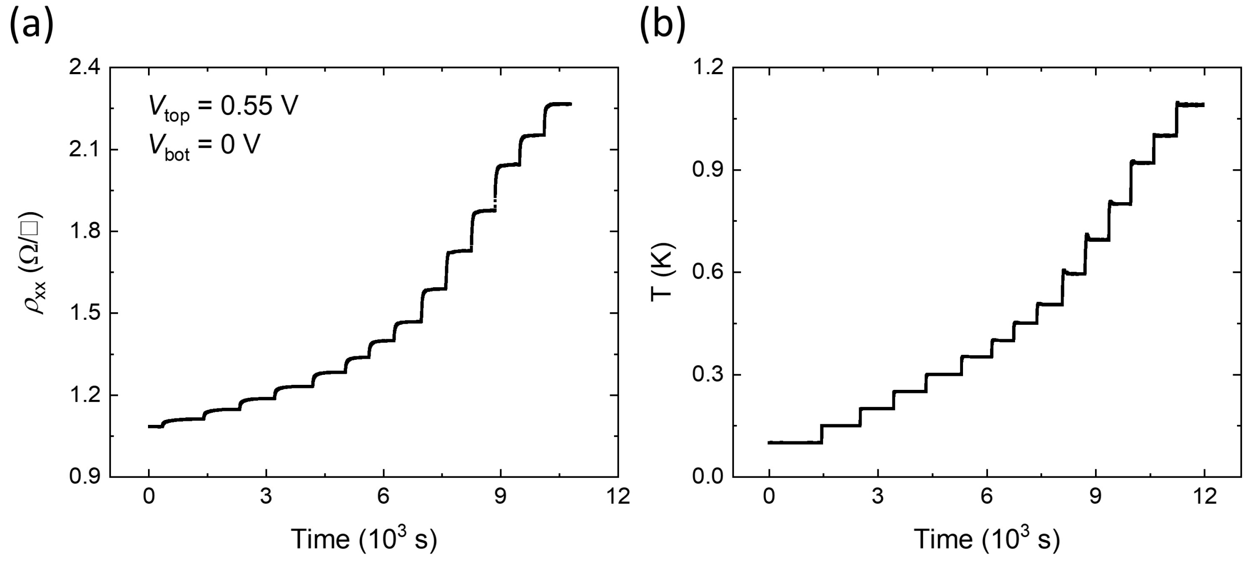


FIG. S2. (a) $\rho_{\text{xx}}$ vs time scan for the variable imbalanced regime at $\nu_{\text{tot}} = 1$ and $n_{\text{tot}} = 9.32 \times 10^{10}$ cm$^{-2}$. (b) Temperature vs time scan. Note that simultaneous plateaus in both panels indicates that the device was given enough time to reach thermal equilibrium.

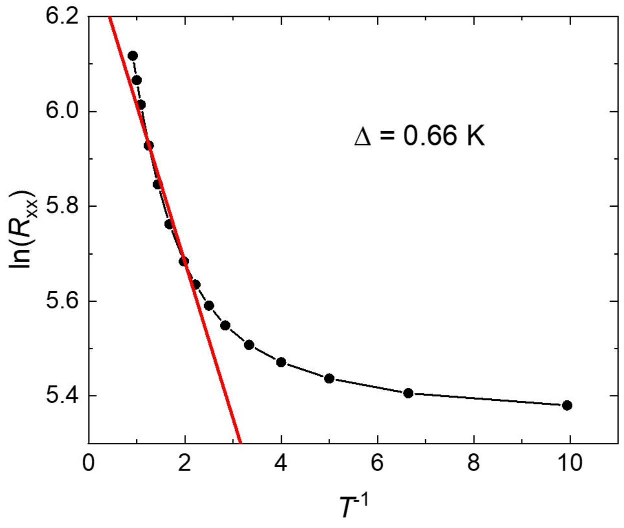


FIG. S3. An Arrhenius plot was formed when the two scans shown in Fig. S2 were combined. $\rho_{xx}$ and T were averaged near the tail end of each plateau. The red line is what the algorithm determined to be the linear portion of the plot.

maximum slope change, only the one with the higher coefficient of determination, $R^2$, is added. This process is repeated until adding a data point changes the slope more than the set threshold. The extracted excitation gap is easily obtained from multiplying the slope by $-2$. Confidence intervals are then found by taking the largest and smallest gap calculated by either adding and/or subtracting an additional point to/from the determined linear activation interval whenever possible. All the initial fitting intervals used are listed in Table S.II. We note that the maximal slope change for each data set was selected to be the lowest value that increased the range of the initial temperature interval. All of the Arrhenius plot fits are shown in Fig. S4, Fig. S5, and Fig. S6 in the next few pages.

TABLE S.II. Linear Fit Parameters

| Data Set | Max Slope % Difference | Starting Temperature (K) | Ending Temperature (K) |
|---|---|---|---|
| Variable Imbalanced ($\nu_{tot} = 1$) | 10 | .5 | .8 |
| Matched ($\nu_{tot} = 1$) | 7 | .4 | .6 |
| Variable Imbalanced ($\nu_{tot} = 2$) | 8 | .5 | .7 |
| Matched ($\nu_{tot} = 2$) | 8 | .4 | .6 |

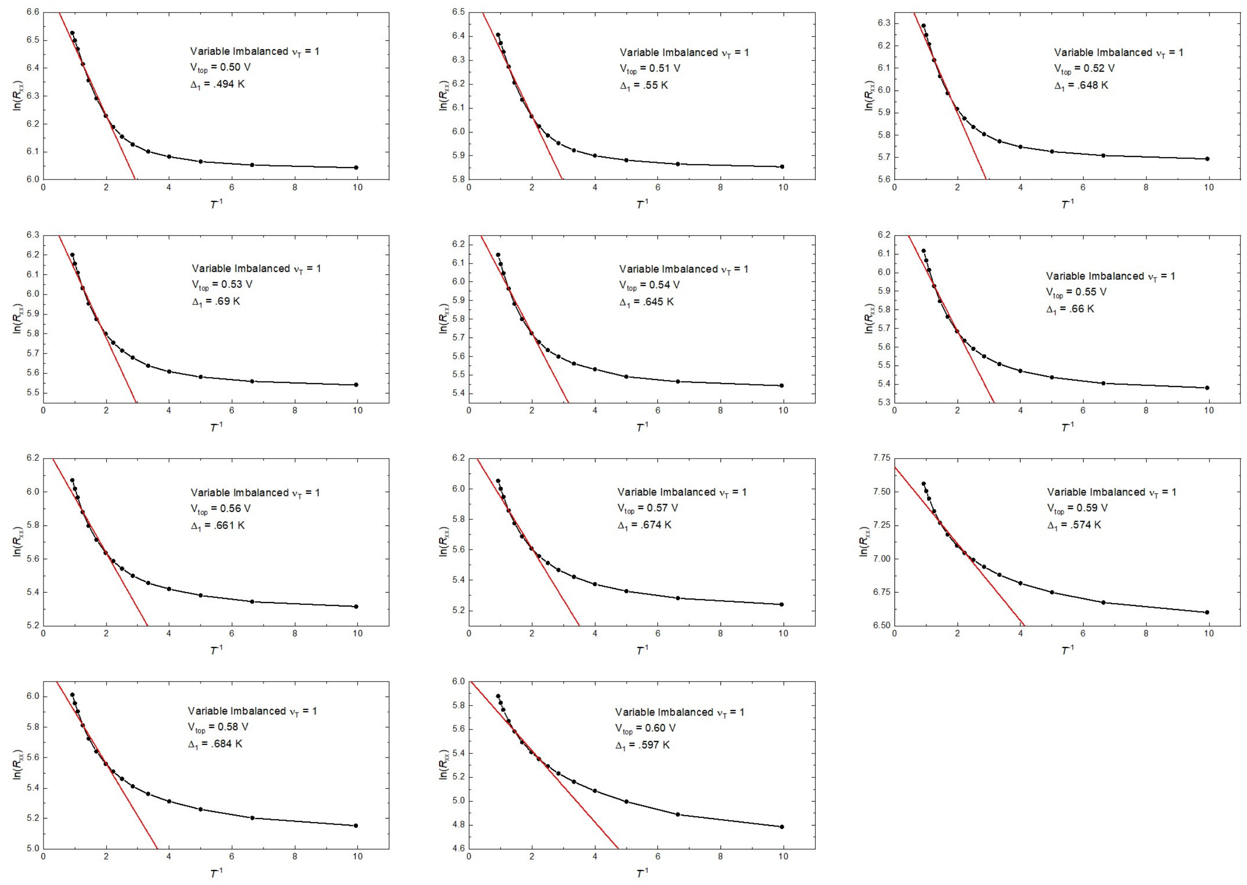


FIG. S4. Arrhenius plots and linear fits for the variable imbalanced density regime at $\nu_{\mathrm{tot}} = 1$.

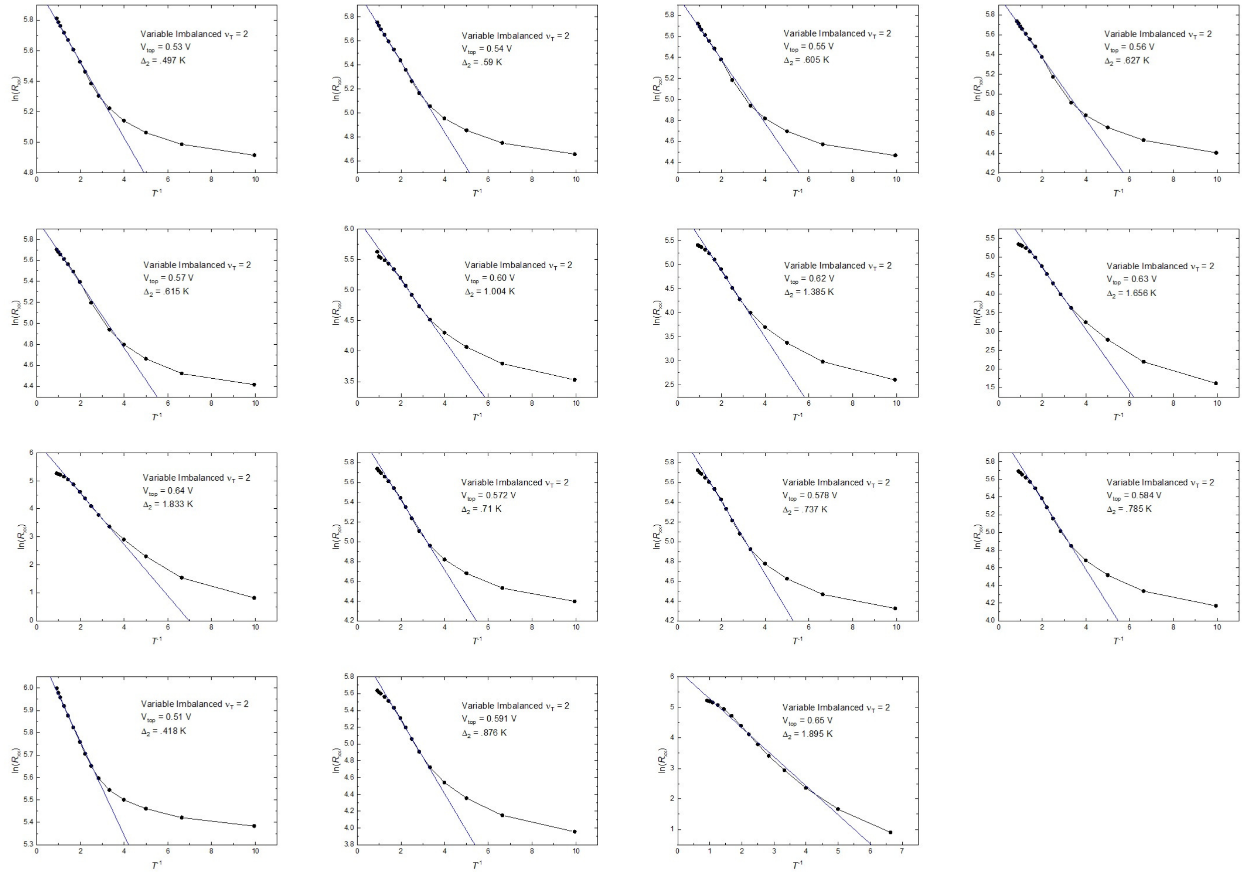


FIG. S5. Arrhenius plots and linear fits for the variable imbalanced density regime at $\nu_{\mathrm{tot}} = 2$.

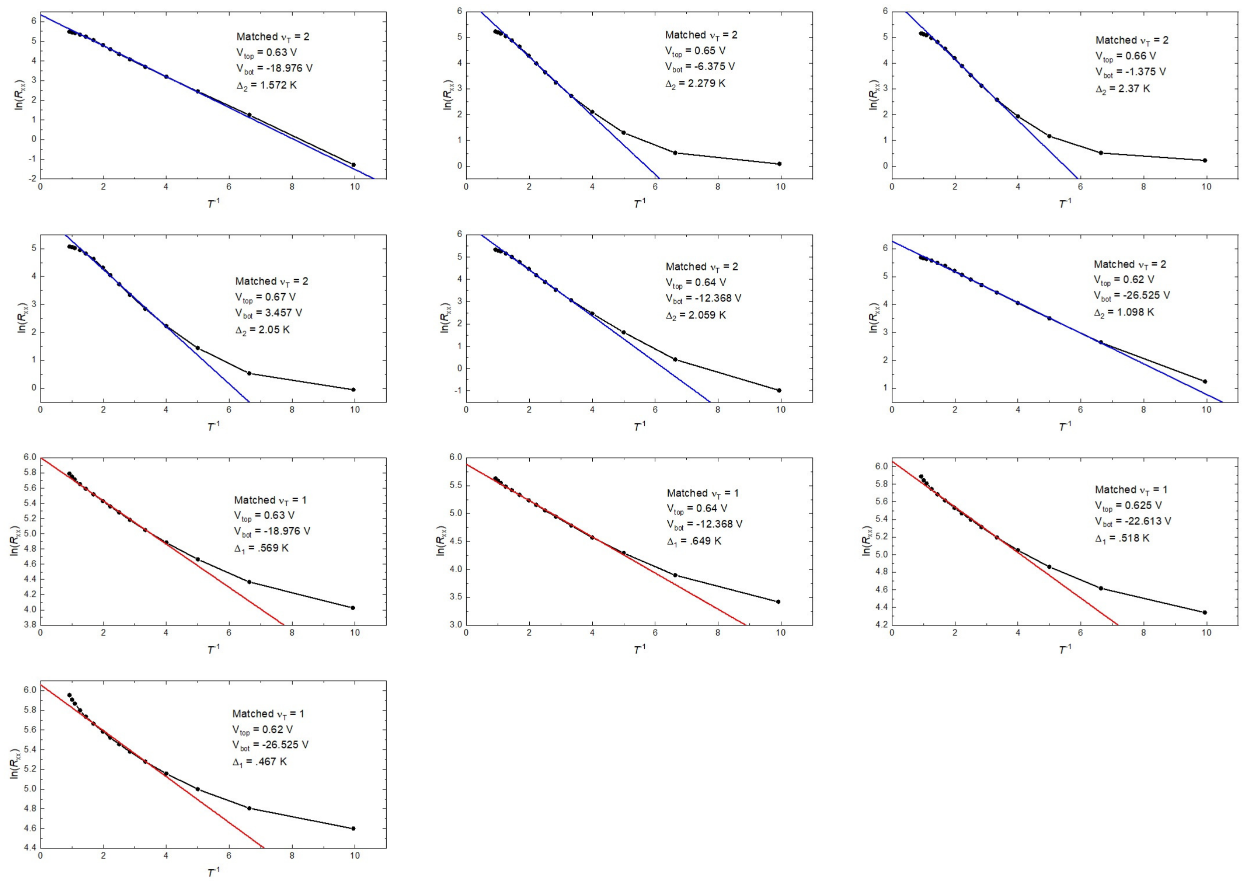


FIG. S6. Arrhenius plots and linear fits for the matched density regime at $\nu_{\text{tot}} = 1$ and $\nu_{\text{tot}} = 2$.

## III. SCHRÖDINGER POISSON SIMULATIONS

An iterative, self-consistent Schrödinger-Poisson (SP) simulation was used in order to determine the conduction band, valence band, energy levels as well as the charge densities in each quantum well, as shown in Fig. S7. To prevent charge accumulation at either interface, the band gaps of the upper and lower half of the heterostructure's top and bottom spacer are artificially increased. Finally, the upper and lower boundary conditions, corresponding proportionally to $V_{\text{top}}$ and $V_{\text{bot}}$, are defined to induce charges in the quantum wells. Functions were coded to allows us to achieve specific densities in each quantum well by systematically modifying both boundary conditions. As stated in Section I, once there is population in both quantum wells, $V_{\text{top}}$ ($V_{\text{bot}}$) strongly affects the densities in the top (bottom) wells in a linear fashion, but also affects the densities in the bottom (top) wells with much less strength. With this in mind, the problem becomes a system of two linear equations with the boundary conditions being the two unknowns. The boundary conditions are adjusted recursively until the target densities are reached in either quantum well, within

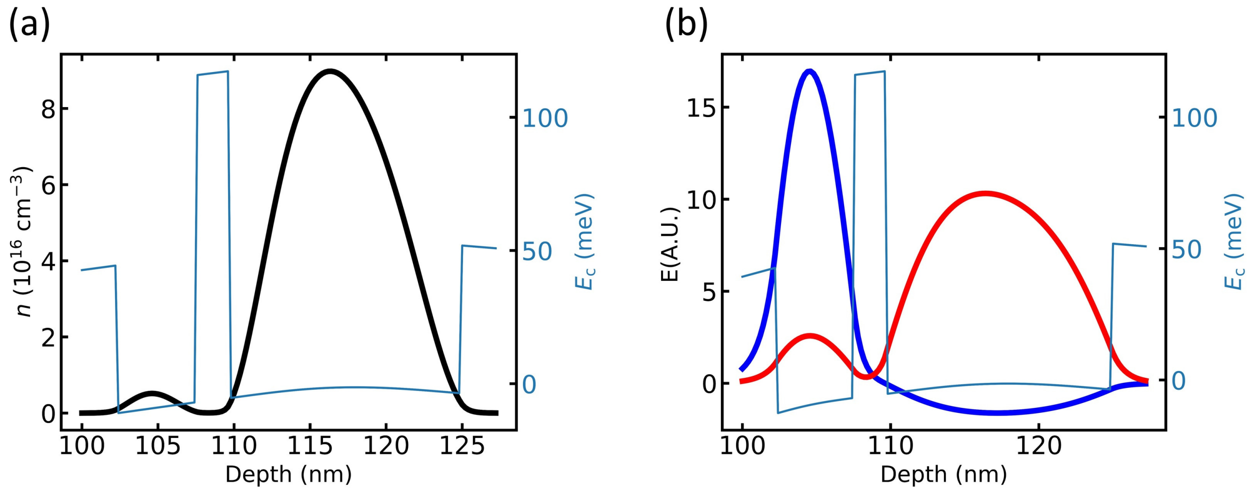


FIG. S7. (a) The device's conduction band (blue) is plotted versus the z-axis at $n_{\mathrm{crossover}}$. We can see that the bottom well is populated with electrons (black) while the top well is starting to populate. (b) The first two energy levels, corresponding to the symmetric and anti-symmetric wavefunctions, are plotted within the quantum wells.

.1%.

As stated in the letter, 4 cases were considered to calculate $\Delta_{\mathrm{SAS}}$. The first variable stems from matching the experimental crossover density, $n_{\mathrm{crossover}}$, achieved during our measurements. One instance used nominal growth parameters and thicknesses but $n_{\mathrm{crossover}}$ could only be achieved by shifting the lower boundary condition, corresponding to a constant offset in the bottom gate voltage. The other instance was able to reproduce the experimental crossover density without utilizing a bottom gate voltage offset by considering a modified structure with a top well width of 3.8 nm, an interlayer barrier of 2.2 nm and a bottom well width of 15 nm. The second variable was necessary to account for possible variations in the interwell barrier heights. Thus, two different interwell barrier heights, $\phi_{\mathrm{b}}$, were used. The first one corresponds to a Ge content of 28.8%, giving $\phi_{\mathrm{b}} = 141.2$ meV; while the other assumes a Ge content of 25.8%, giving $\phi_{\mathrm{b}} = 122.8$ meV. Together, there are four simulated cases. In general, $\phi_{\mathrm{b}}$ has a limited effect on the electronic densities of the wells but has a noticeable effect on $\Delta_{\mathrm{SAS}}$. We show the simulated $\Delta_{\mathrm{SAS}}$ values for all four cases in the following figure.

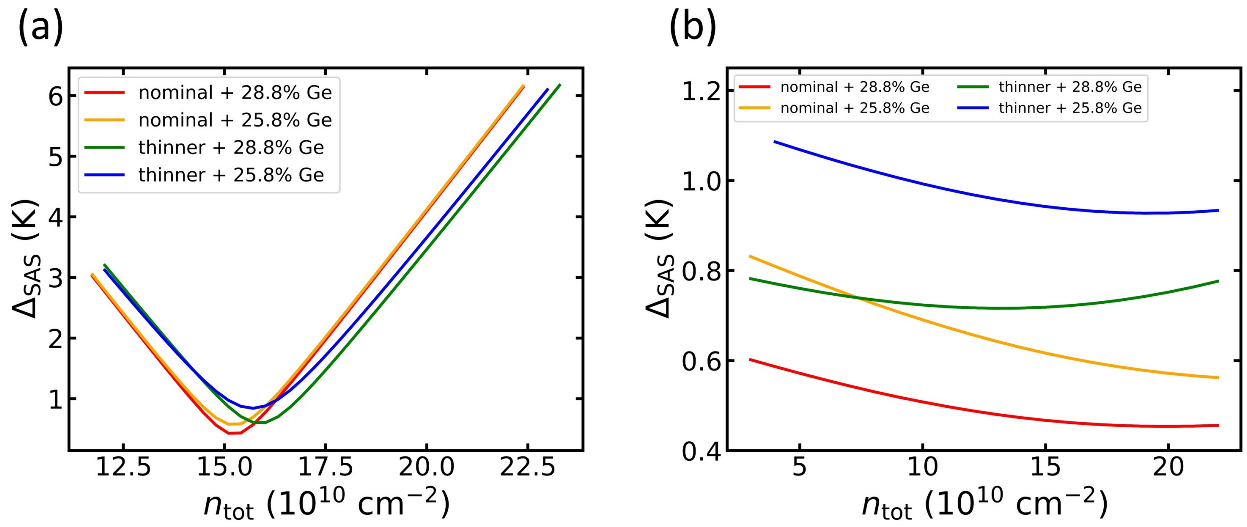


FIG. S8. (a) $\Delta_{SAS}$ is plotted, showing the differences across the four different cases in the variable imbalanced density regime. "Nominal" corresponds to as grown parameters while "thinner" corresponds to a thinner top quantum well width but a slightly thicker interwell barrier. (b) $\Delta_{SAS}$ is shown for the matched density regime for all four cases.
